# Supplementary material for: Predicting Relationship Labels and Individual Personality Traits from Telecommunication History in Social Networks using Hawkes Processes
Source: arXiv:2009.02032 source file (2023-01-25)
Supplement: Supplementary file 1 [file appendix.tex]

\clearpage
\appendix
% \onecolumn

\section*{Supplementary information}
\vspace*{.3cm}

This document is accompanying the submission \textit{\titlename}.
The information in this document complements the submission, and it is presented here for completeness reasons. 
It is not required for understanding the main paper nor for reproducing the results.

\section{Generalization performance for Hawkes kernels}
\cref{fig:kernelComparison} shows the resulting negative holdout log-likelihood (lower is better), summarized as boxplots for each kernel and each dataset.

%!TEX root = ../main.tex
% 
\begin{figure}[h]
	\centering
	\includegraphics[width=0.45\textwidth]{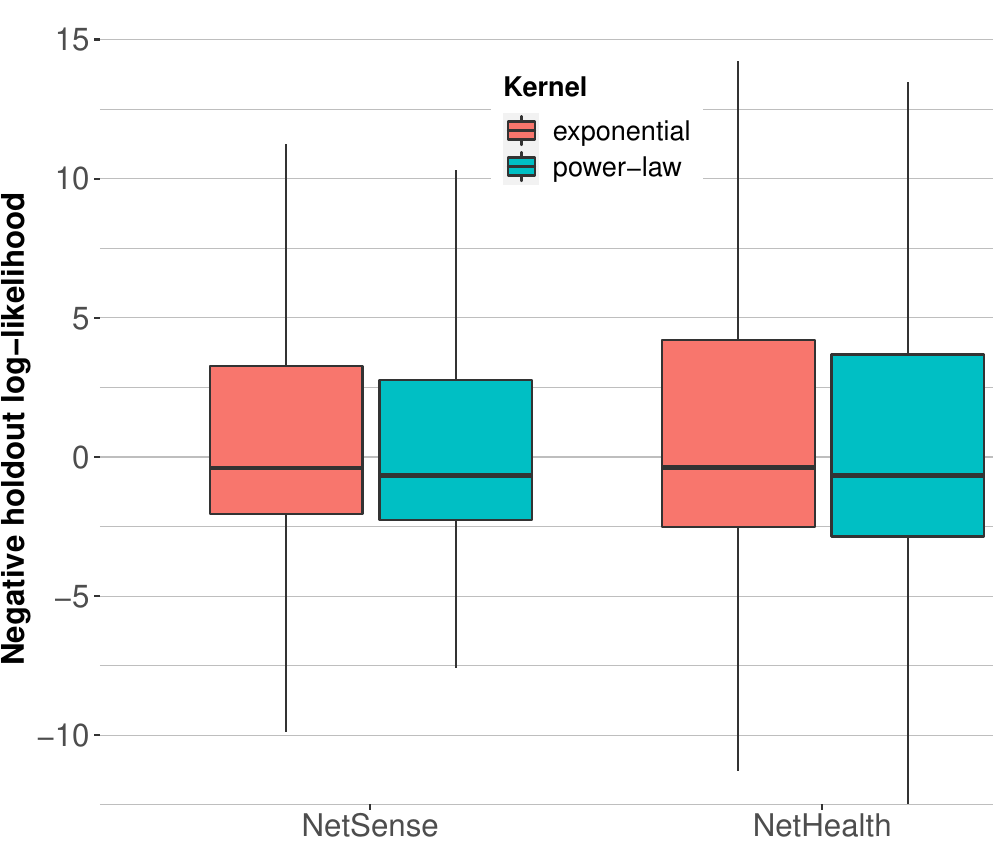}
	\caption{
		Generalization performance for Hawkes kernels.
		The boxplots summarize the temporal holdout log-likelihood per event, for $\phi_{EXP}(t)$ and $\phi_{PL}(t)$ -- the exponential and the power-law kernels.
		Lower is better.
	}
	\label{fig:kernelComparison}
	\vspace*{-.5cm}
\end{figure}

\section{Performance of predicting relationships types}
\cref{fig:relationship-classification-full} shows the relationship prediction results obtained by all tested classification algorithms: Random Forest, SVM, and XGBoost.
%!TEX root = ../main.tex
% 
\begin{figure*}[h]
	\centering
	\includegraphics[width=1\textwidth]{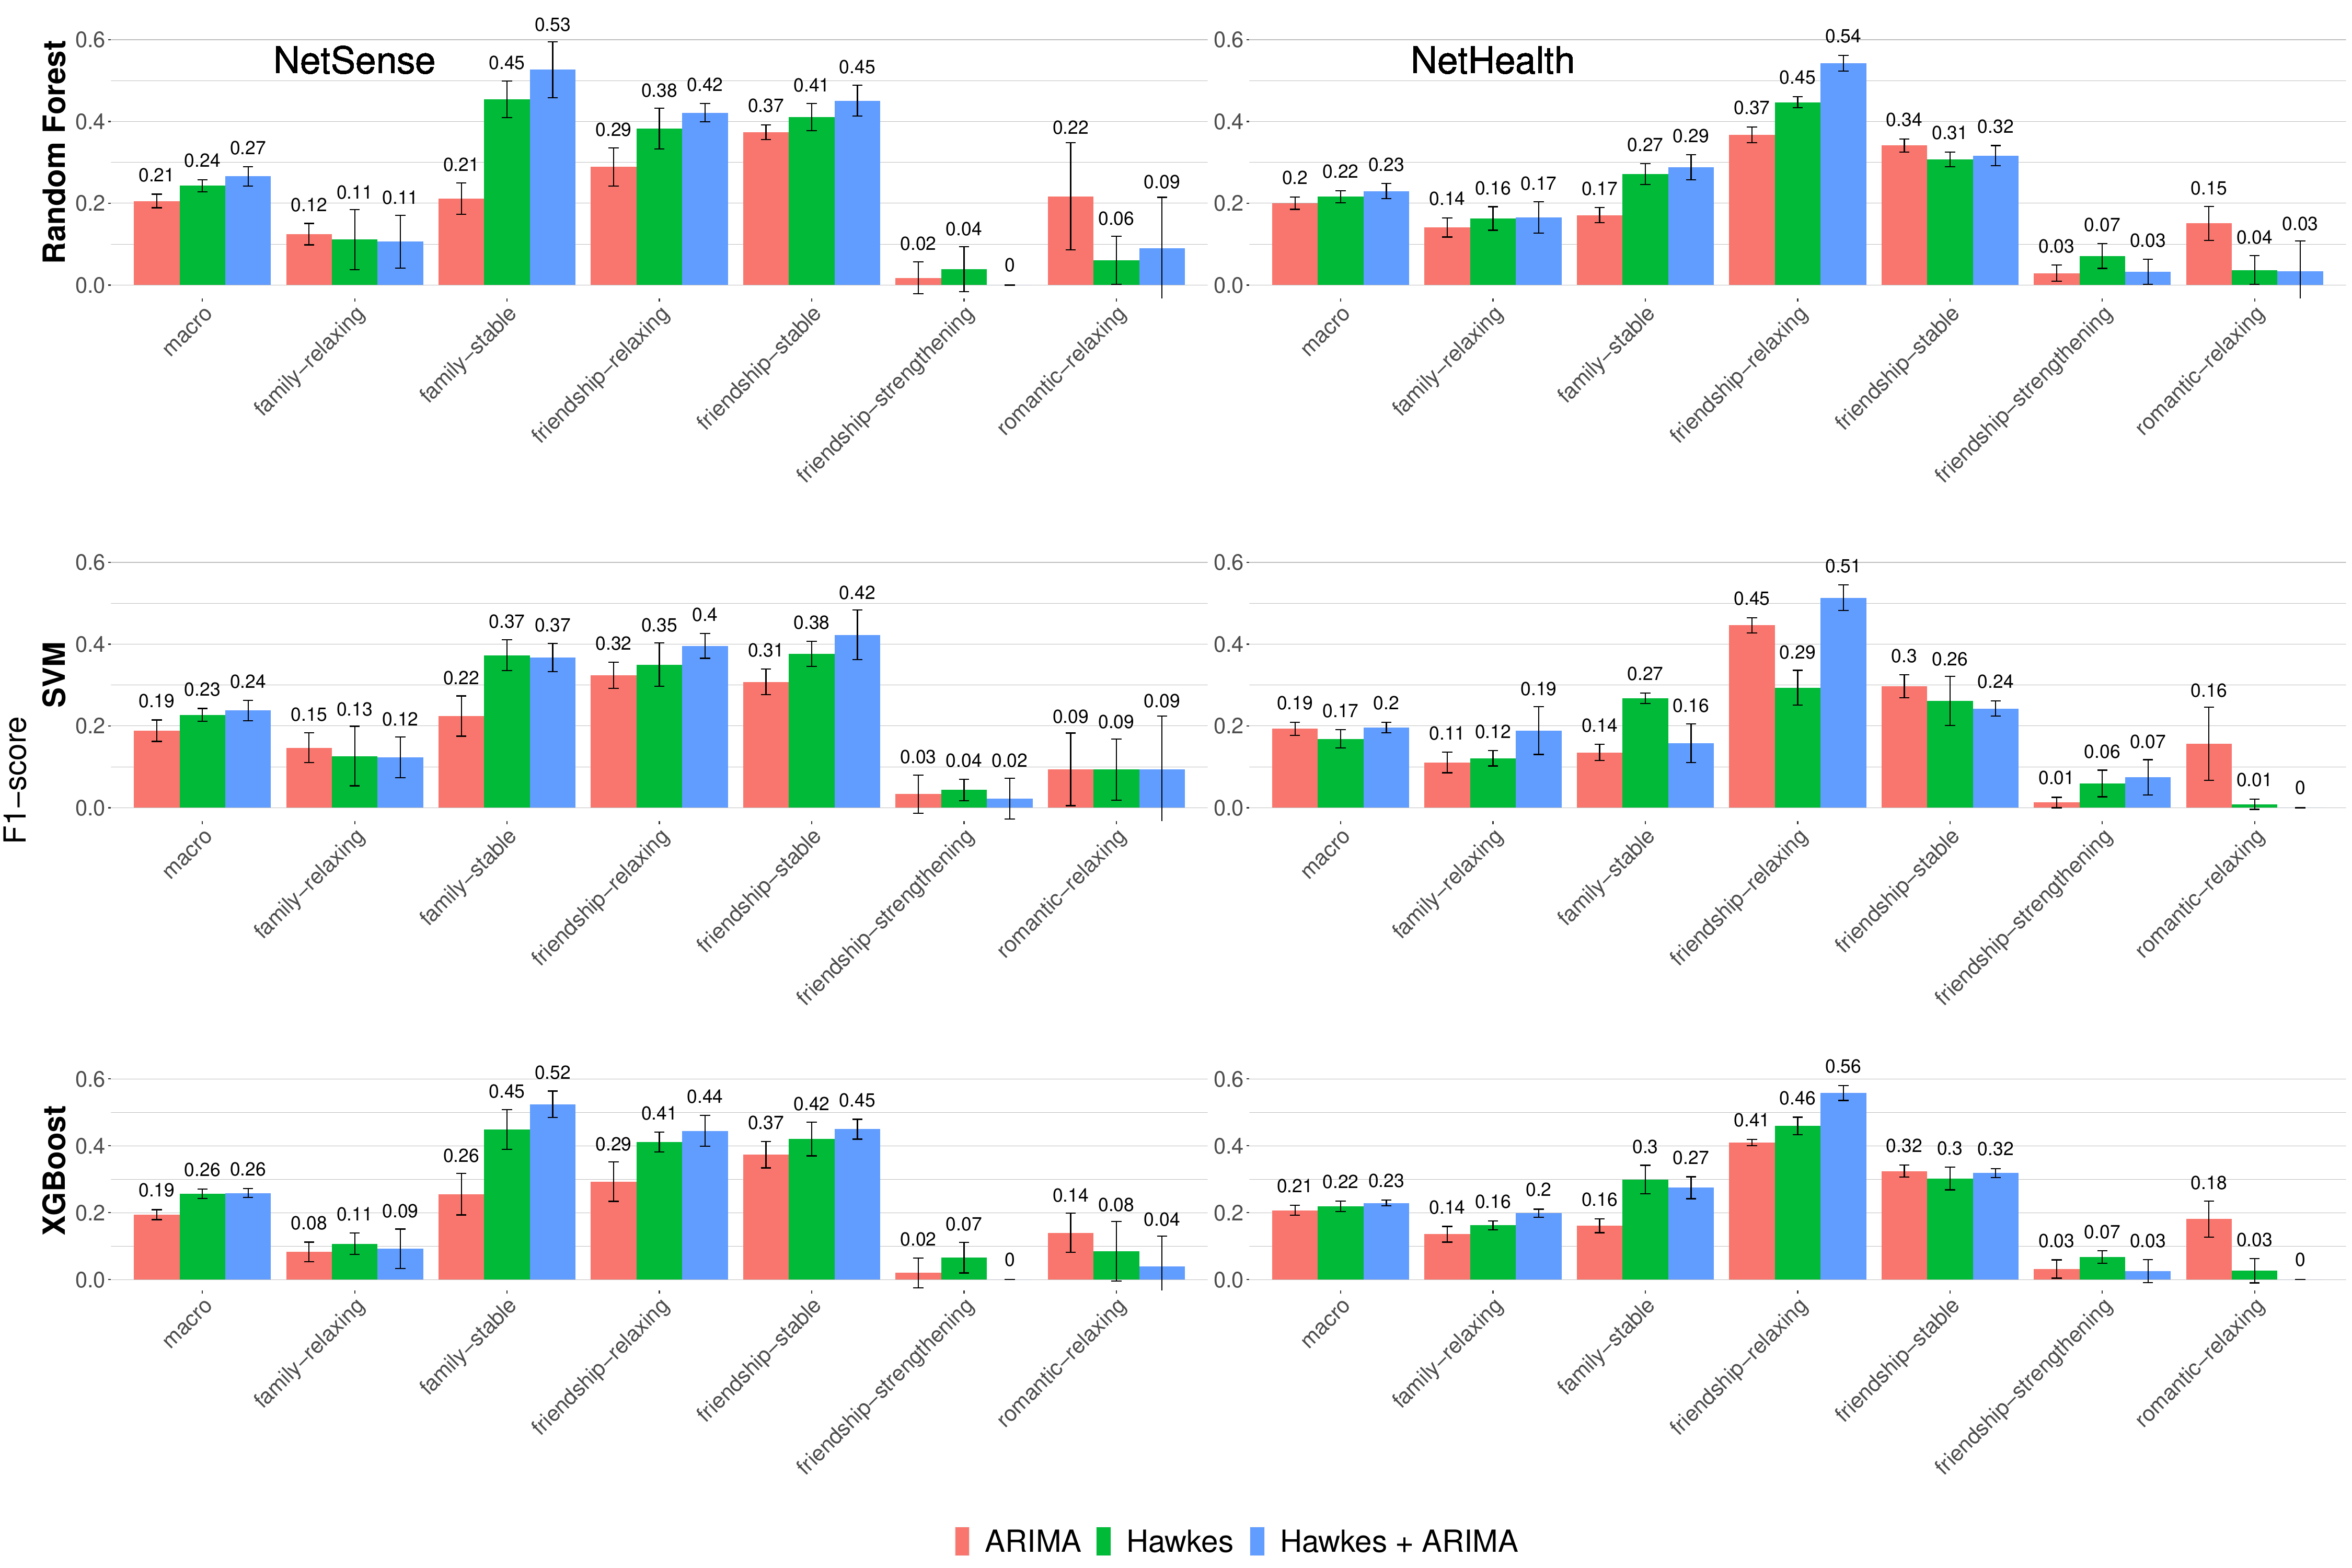}
	\caption{Performance of predicting relationship types using the call activity modeled using Hawkes processes and ARIMA (higher is better).}
	\label{fig:relationship-classification-full}
\end{figure*}

\section{Detect temporal change points}
\label{subsec:temporal-change-points}

Here, we leverage the finding that relation types have consistent profiles in the space of Hawkes parameters.
We propose a method to detect if a relation change occurred between consecutive surveys.

% The classification of dynamic types of relations turned out to be a difficult task, so we attempted to predict whether the change itself would occur. 
% Using the history of outbound callings between a pair of users, we tried to predict whether it is possible to predict the change itself without specifying the type of relationship. 
% We have proposed a novel method for temporal change detection in a dynamic relationship based on the Hawkes process.
% 
\noindent\textbf{Methodology.}
Our method uses the change in the holdout log-likelihood.
Intuitively, when a relation transitions to a new relation type, the parameters fitted on the previous type would poorly describe the new calling dynamics.
We set up a holdout log-likelihood measurement exercise to detect this change.
\cref{fig:detectingTemporalChangePoints} schematically shows the method.
The top axis shows the call series timeline.
We use the surveys filled in by the caller (denoted as $S_l$) to discretize the timeline; at each $S_l$, the caller defines the type of relation with the call receiver.
In the example in \cref{fig:detectingTemporalChangePoints}, the relation type changed between $S_i$ and $S_{i+1}$ -- say from \emph{significant other} to \emph{friend}.
I.e., the relation was labelled as \emph{significant other} $\forall S_l, l \leq i$ and as \emph{friend} at $S_{i+1}$.
We detect the transition as shown in the lower two axes.
First (middle axis, shown in blue), we train a Hawkes model on the period $[0, S_{i-1})$, and we compute the holdout log-likelihood on the period $[S_{i-1}, S_{i})$.
The relation is the same both on the train and holdout period, and the fitted model should have a good generalization performance.
Second (lower axis, shown in green), we fit the Hawkes model on the period $[0, S_{i})$, and we compute the holdout on $[S_{i}, S_{i+1})$.
Given that the relationship changes before $S_{i+1}$, we expect the holdout log-likelihood (per event) on $[S_{i}, S_{i+1})$ to be significantly lower than $[S_{i-1}, S_{i})$.

%!TEX root = ../main.tex
%
\begin{figure}[h!]
	\centering
	\includegraphics[width=0.45\textwidth]{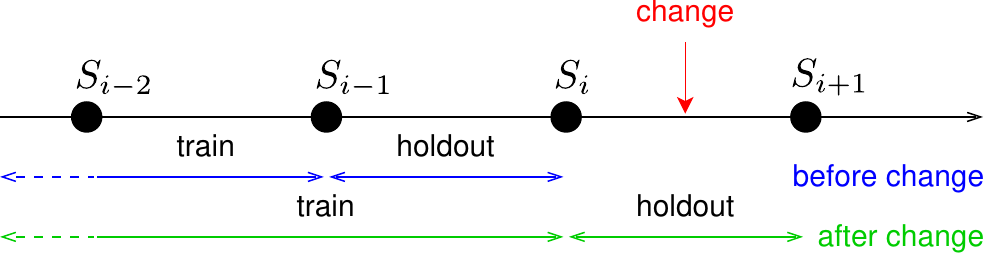}%
	\caption{
		Schema for detecting changes in relationships. 
		% The relationship changed between the completion of the second and third surveys by the student. We detect the change by comparing the holdout negative log-likelihood value of the Hawkes processes fitted before and after the change.
		We train and test before the change (shown in blue) and after (shown in green), and we compare the holdout likelihoods.
	}
	\label{fig:detectingTemporalChangePoints}
%	\vspace*{-.3cm}
\end{figure}%

\noindent\textbf{Results.}
Our method imposes several restrictions.
First, it requires that students fill in at least three surveys (though this can be reduced to only two surveys by creating an artificial ``survey'' before the first one).
Second, the change should occur after the second survey.
Third, it requires that the call history extends throughout all considered periods.
When accounting for the restrictions, we are left with 442 call histories for \Netsense and 1888 for \Nethealth across four dynamic relationship types (shown in \cref{tab:wilcox}).
We perform a paired Wilcoxon signed-rank test to determine the statistical significance of the difference between the log-likelihood before and after the change.
\cref{tab:wilcox} shows the p-value of the test (conf. level $= 95\%$) for each relationship type and the effect size (measured using Cohen's $d$~\cite{cohn1988statistical}) to account for the variability in sample sizes. Visibly, for \Nethealth, \emph{family-relaxing} and \emph{friendship-relaxing} are both statistically significant (p-value $\ll 0.001$), with small effect sizes.
For \Netsense, \emph{friendship-relaxing} the effect size is negligible; however, the difference appears statistically significant -- probably due to the large size of the class.
For all other relationship types, the difference is not statistically significant.
These results show that we can use the fitted Hawkes processes to detect the change point for particular relationship types.

%!TEX root = ../main.tex
%
\begin{table}[h!]
	\caption{
		% Detect temporal change points in relationships using the 
		Wilcoxon signed-rank test (conf. level = 0.95) and Cohen's d for detecting relationship change point.
	}
	\label{tab:wilcox}
	\small    
	\setlength{\tabcolsep}{0.1pt}
	\begin{tabular}{p{2.5cm}|ccc|ccc}
		\toprule
		\multirow{2}{*}{\textbf{Type}}&\multicolumn{3}{c|}{\textbf{\Netsense}}&\multicolumn{3}{c}{\textbf{\Nethealth}}\\
		&P-value&Effect size&Inst.&P-value&Effect size&Inst.\\
		\midrule
		family-relaxing & 0.51 & 0.23 & 65 & \textbf{5.09e-07} & \textbf{0.25} & 313\\
		friendship-relaxing & 9.41e-07 & 0.04 & 370 & \textbf{4.62e-28} & \textbf{0.14} & 1532\\
		friendship-strength. & 0.25 & 0.71 & 4 & 0.47 & -0.40 & 30\\
		romantic-relaxing & 1 & 0.05 & 3 & 0.37 & 0.56 & 13\\
		\bottomrule
	\end{tabular}
	\vspace*{-.3cm}
\end{table}

\section{Inferring psychometric traits - RMSE performance}
\cref{fig:rmseBig5} shows the Big5 traits prediction performance measured using the RMSE (lower is better) for \Netsense and \Nethealth.

%!TEX root = ../main.tex
% 
\begin{figure*}[h!]
	%% MAR: align subfigs by height
	\centering
	\setkeys{Gin}{height=0.205\textheight}
	\subfloat[]{
		\includegraphics{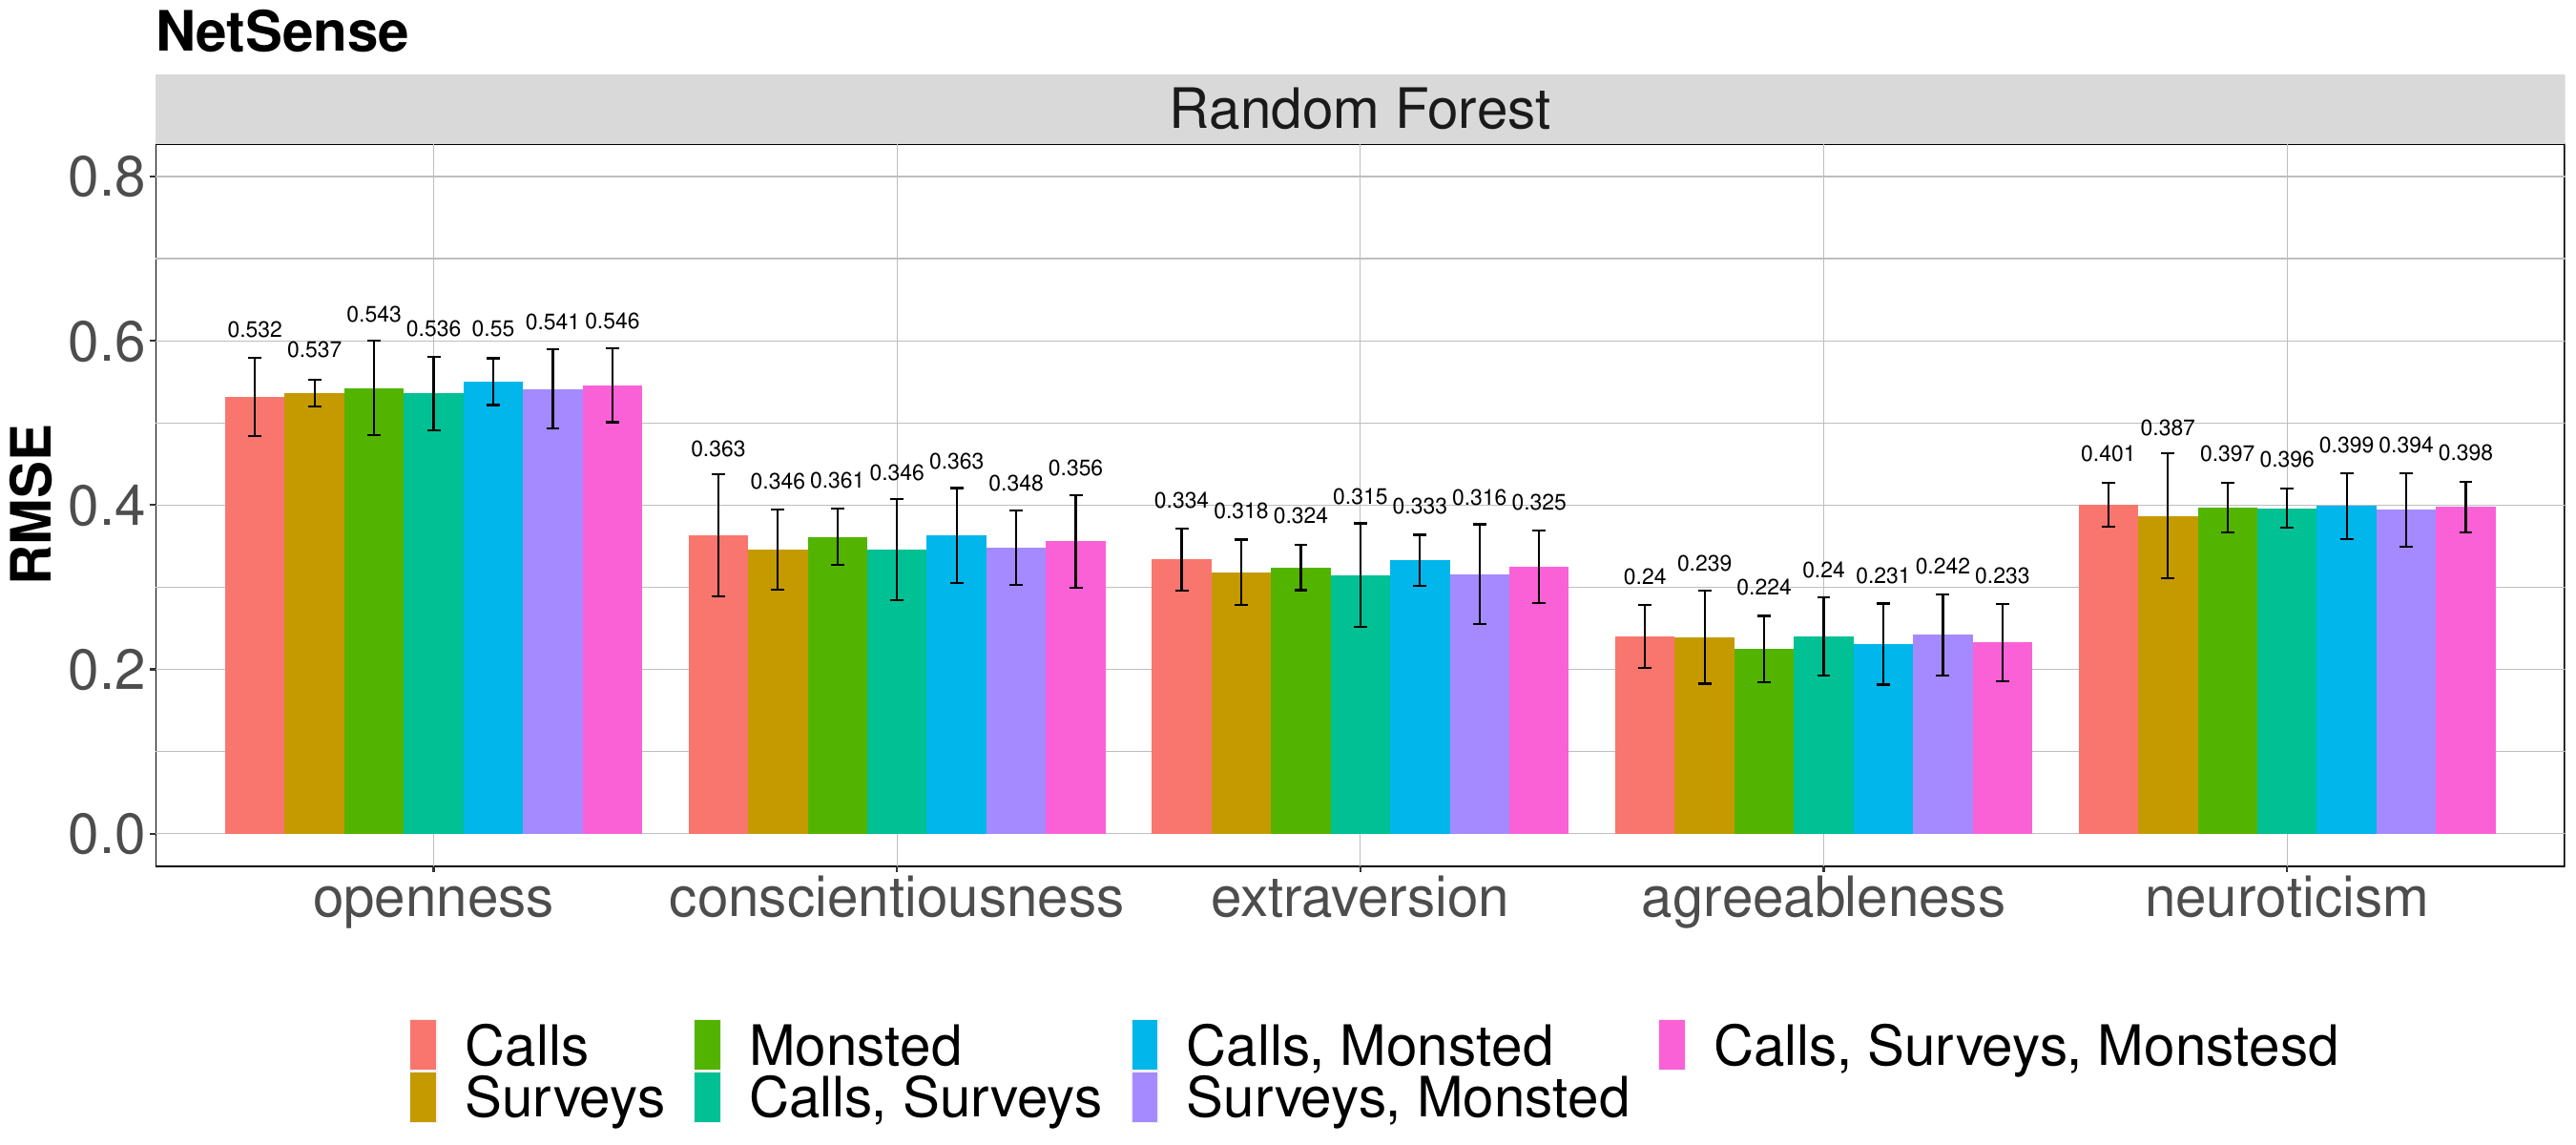}
		\label{fig:rmseBig5-1}
	}%
	
	\subfloat[]{
		\includegraphics{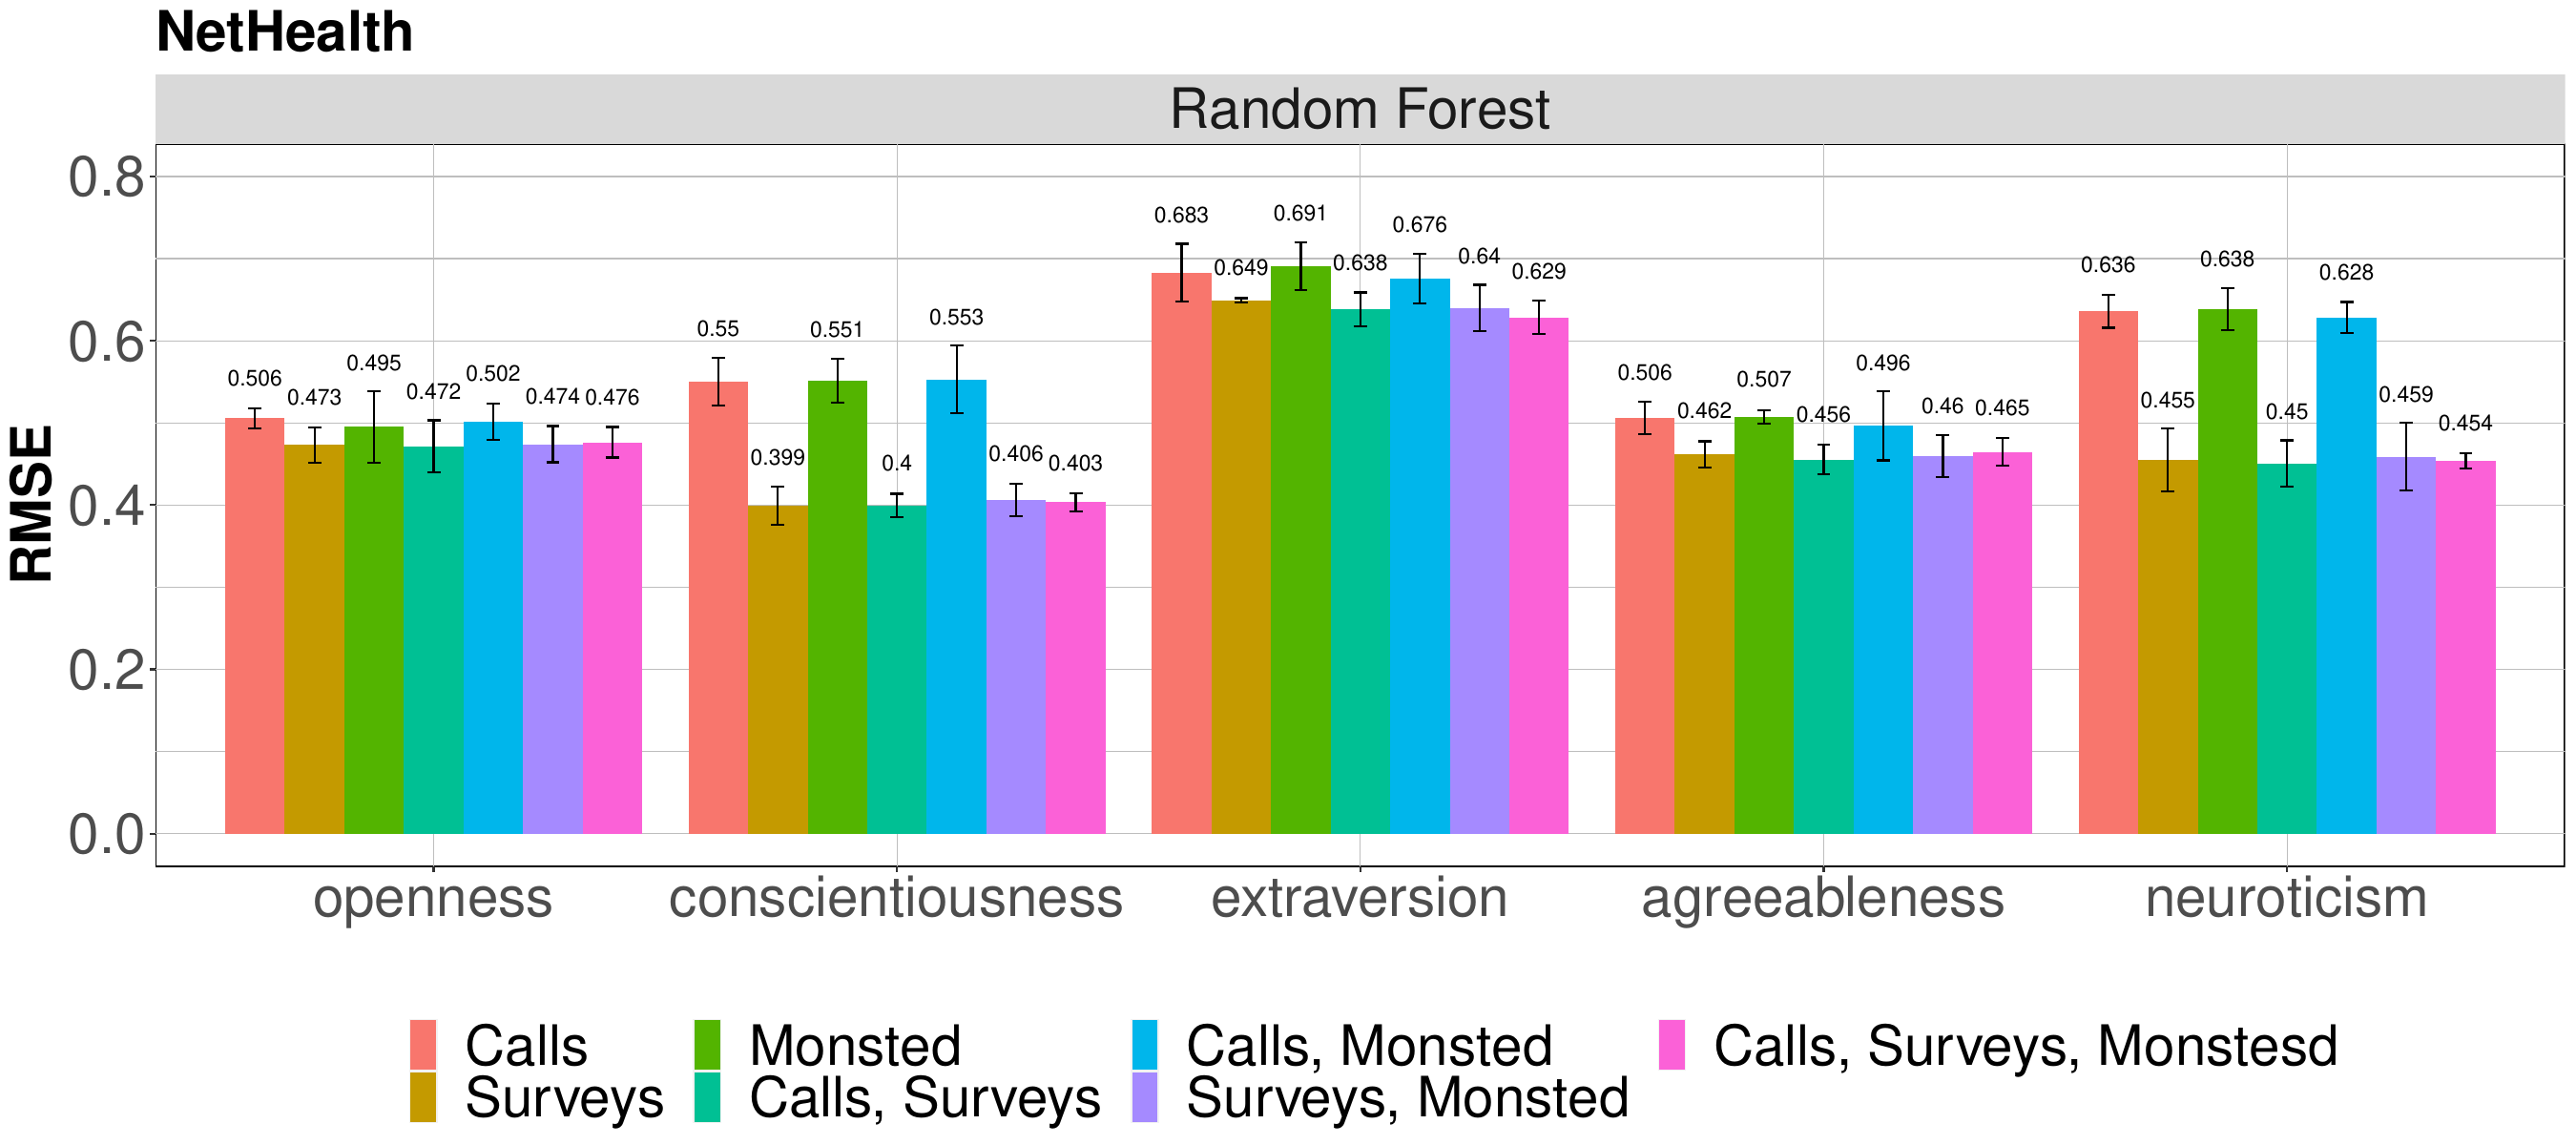}
		\label{fig:rmseBig5-2}
	}%
	\caption{
	    \textbf{Big5 traits prediction performance measured using the RMSE.}
		Students are described using features built on two data sources (calls and filled-in surveys).
		For calls, we describe the users using our Hawkes-model embedding (Hawkes) and using a recent baseline~\cite{Monsted2018} (Monsted).
		We also test combinations of feature sets.
	}
	\label{fig:rmseBig5}
\end{figure*}

\section{Additional related work}

This section presents, for completeness, more related work relevant to this work.
First, we review theoretical and empirical research on the emergence and properties of contact networks.
Second, we glance over other works that use mobile phone data.

\noindent\textbf{Theoretical and empirical research on the emergence of contact networks and their properties.}
The connection between bursty behavior and power-law distributions of activity in social networks has been known for more than a decade.
Bursts in human and natural activities are highly clustered in time or space, suggesting that these activities are influenced by previous events within the social or natural system~\cite{Kim2018}.
Barab{\'{a}}si~\cite{Barabasi2005} proposed a decision-based queuing process in which individuals execute tasks based on some perceived priority.
The emergence of power-law in social systems has been theoretically studied for movie ratings~\cite{Kim2018}, and the view count series of Youtube videos~\cite{Crane2008}.
Further connections have been shown between the arrival of events in contact networks and the structure of the network~\cite{takaguchi2012importance} 

A number of empirical studies were set up to infer the link between contact events and the structure of the inferred network.
Lee et al~\cite{Lee2018} build a study in which they give a group of students mobile phones, and they survey them five times a year.
They find that consistent deviations from expected behavior are crucial for identifying well-established underlying social relationships.
Raeder et al~\cite{raeder2011predictors} use the same \Netsense dataset as our work to predict edge decay in social contact networks, i.e., whether an edge that was active in one time period continues to be so in a future time period.
Radio Frequency Identification devices that assess mutual proximity were used by Cattuto et al~\cite{Cattuto2010a} to study offline contact networks. 
The study found an interesting super-linear behavior, which indicates the possibility of defining super-connectors both in the number and intensity of connections.

Our own study relies on contact events along the edges of a social graph. 
Still, we do not use these to study the network, but rather what information these uncover concerning the users themselves.

\textbf{Other applications.}
There are a large number of works that use mobile phone data to learn and predict other quantities.
While these are only marginally related to our work, we present some of them for completeness reasons.
For example, Gonzalez et al~\cite{Gonzalez2008} used the GPS location of the mobile phones to analyze mobility patterns for six months and found that despite the diversity of their travel history, humans follow simple, reproducible patterns.
{\'{O}}skarsd{\'{o}}ttir et al~\cite{Oskarsdottir2017} use social media traits to predict customer churn (i.e., whether customers will leave the mobile network for one of the competitors).
The same problem is addressed by Backiel et al~\cite{Backiel2014}, who also use network operator information (such as last reload date, number of calls in the last 60 days, card swapped in 30 days) in addition to simple features relating to the network of callers.
Furthermore, Steele et al~\cite{Steele2017} and Smith-Clarke et al~\cite{Smith-Clarke2014} use aggregate data from mobile operators to model the spatial distribution of poverty in a population, while Soto et al~\cite{Soto2011} use aggregated cell phone records to identify the socioeconomic levels of a population.
Finally, Bach et al~\cite{Bach2019} use mobile usage data to predict voting outcomes.
The survey by Calabrese et al~\cite{Calabrese2014} inventories a series of features constructed for analyzing telecom data, but unlike our work, they do not fit Hawkes point process.
